# Supplementary material for: On the Sample Complexity and Metastability of Heavy-tailed Policy Search in Continuous Control
Source: arXiv:2106.08414 source file (2023-01-02)
Supplement: Supplementary file 1 [file Appendix_E_uncorrected.tex]

%!TEX root = root.tex

%%%%%%%%%%%%%%%%%%%%%%%%%%%%%%%%%%%%%%%%%%%%%%%%%%%%%%%%%%%%%%%%%%
%%%   S   E   C   T   I   O   N   %%%%%%%%%%%%%%%%%%%%%%%%%%%%%%%%
%%%%%%%%%%%%%%%%%%%%%%%%%%%%%%%%%%%%%%%%%%%%%%%%%%%%%%%%%%%%%%%%%%
%%%%%%%%%%%%%%%%%%%%%%%%%%%%%%%%%%%%%%%%%%%%%%%%%%%%%%%%%%%%%%%%%%%%%%%%%%%%%%%%
\section{Proof for Theorem \ref{Theorem:Exit time}: First Exit time Analysis for Heavy-tailed Policy Gradient}
\label{Proof:exittime}
\blue{This is a newly added section. I need to merge it with the previous section based on comments.} 
\begin{proof}
 We start along the lines of \cite{simsekli2019tail, thanh2019first, tzen2018local}  and relate  the proposed setting of  \eqref{eqn:SGD_L} to the continuous SDE of \eqref{eqn:SGD_L1}.  
 We define a domain, $\mathcal{G}$ with respect to $\bar{\bbtheta}_i$  such that 
\begin{align}
\mathcal{G}:= \{ \mathbb{\bbtheta} \in \mathbb{R}^d: \| \bbtheta - \bar{\bbtheta}_i\| \leq a+\xi \}
\end{align} 
where, $a, \, \xi >0$. Let us first  formally define the exit time for both discrete and continuous  processes. 
%Let  $\bbtheta_t =\bbtheta_k, \, t=k\eta=0$ (both discrete and continuous processes are initialized with $\bbtheta_0$) and the time required  to exit the basin $[0, a+\xi]$ by the process \eqref{eqn:SGD_L1} is defined by 
%
\begin{align}\label{exit_contins}
%
%& \hat{\tau}_{\xi,a} (\epsilon) \triangleq \inf \{ t \geq 0:  \| \bbtheta_t -\bar{\bbtheta}\| \notin [0, a + \xi]  \}, \\
%& \green{
\hat{\tau}_{\xi,a}(\epsilon) \triangleq \inf \{ t \geq 0:  \bbtheta_t \notin \mathcal{G}   \}
\end{align}
and the time at which the discrete time process \eqref{eqn:SGD_L} exits $\mathcal{G}$ is given by 
\begin{align} \label{eqn:taudisccrt}
%
%& \bar{\tau}_{\xi,a} (\epsilon) \triangleq \inf \{ K \in \mathbb{N} :  \| \bbtheta^k -\bar{\bbtheta}\| \notin [0, a + \xi]  \} \\
%& \green{
\bar{\tau}_{\xi,a}(\epsilon) \triangleq \inf \{ K \in \mathbb{N} :   \bbtheta^K  \notin \mathcal{G}   \}
\end{align}
Note that $\bar{\tau}(\cdot)$ represents the exit time of discrete-time process $\bbtheta^k$, whereas $\hat{\tau} (\cdot) $ denotes that of continuous-time stochastic process $\bbtheta_t$. We define the set of $K$ points, $k=1 \ldots, K$  obtained  from  \eqref{eqn:SGD_L} which are at a maximum distance of $a$ from the local minima (\blue{change to maxima once analysis is finalized} ) of interest, $\bar{\bbtheta}_i$ is defined as 
\begin{align}\label{eqn:aset}
A \triangleq \{  (\bbtheta^1, \ldots, \bbtheta^k): \max_{k \leq K} \| \bbtheta^k -\bar{\bbtheta}_i \| \leq a    \} 
\end{align}
Next we define a set $N_a$ as the neighborhood in Euclidean distance centered at $\bar{\bbtheta}$:
\begin{align}\label{eqn:Na}
N_a \triangleq \{ \bbtheta \in \mathbb{R}^d: \| \bbtheta - \bar{\bbtheta}_i \| \leq a \}.
\end{align}
As we initialized both discrete and continuous process at $\bbtheta_0$, processes defined by  \eqref{eqn:SGD_L} and \eqref{eqn:SGD_L1} are close enough if both of their   exit times from $N_a$ are close, ie.,  $\mathbb{E}_{\bbtheta_0}\left[ \| \bbtheta^{k} - \bbtheta_{k\eta} \|  \right]  \leq \frac{\delta}{2}$, let say the upper bound is $\delta/2$.  Using Markov's inequality, the above statement can be expressed in the language of probability as 
\begin{align} 
\mathcal{P}^{\bbtheta_0} \left( \| \bbtheta^{k} - \bbtheta_{k\eta} \| > \epsilon    \right) \leq \frac{\EE_{\bbtheta_0}\left[  \| \bbtheta^{k} - \bbtheta_{k\eta} \| \right] }{\epsilon} \frac{}{}   \leq \frac{\delta}{2}
\end{align} 
the above expression defines the probability that $ \| \bbtheta^{k} - \bbtheta_{k\eta} \| > \epsilon$ given $\bbtheta^0 = \bbtheta_0$ as $\delta/2$.  For the time being, we assume constant step-size $\eta$  and consider the linearly  interpolated version of \eqref{eqn:SGD_L} given by 
\begin{align}\label{eqn:SGDint}
d \hat{\bbtheta}_t = b(\hat{\bbtheta}_t) dt  + \epsilon dL_{\alpha}^t, 
\end{align}
Note that the unit vector direction of perturbation is absorbed in to $dL_{\alpha}^t$ (cf. \eqref{eqn:Levygeneric}).  Here, $\hat{\bbtheta} = \{\hat{\bbtheta}_t\}_{t \geq 0}$ denotes the whole process with drift term, $b$ defined as 
\begin{align*}
b(\hat{\bbtheta}_t) \triangleq - \sum_{k=0}^{\infty} \nabla F(\hat{\bbtheta}_{k \eta})  \mathbb{I}_{[k\eta , (k+1) \eta )} (t). 
\end{align*}
{The above expression can also be expressed as $$  b(\hat{\bbtheta}_t) \triangleq - \frac{1}{1-\gamma} \sum_{k=0}^{\infty} \EE_{s, a \sim \rho_{\hat{\bbtheta}_{k\eta}} } [\nabla \log \pi_{\hat{\bbtheta}_{k\eta}} Q_{\pi_{\hat{\bbtheta}_{k\eta}}}(s,a)] \mathbb{I}_{[k\eta , (k+1) \eta )} (t).$$ }
Here, $\mathbb{I}$ denotes the indicator function such that $\mathbb{I} = 1 $ if $t \in [k\eta, \, (k+1) \eta)$. First exit time of a continuous SDE \eqref{eqn:SGD_L1}   is summarized in Theorem \ref{th:2} \cite{imkeller2006first}.  We first establish the connection between   the exit times of \eqref{eqn:SGD_L} and \eqref{eqn:SGD_L1} and obtain the results for the proposed heavy-tailed setting as function of its continuous equivalent.\\
Given the continuous time instant  t, $t=k\eta$ and let $\bbtheta_{k\eta} \in N_a$,  the following events can happen
\[
\bbtheta^k \begin{cases}
 \in N_a & \textrm{with} \, \mathcal{P} ( \bbtheta^{k} \in N_a) \\
  \notin N_a:  \|\bbtheta^k -\bbtheta_{k\eta}\| >\epsilon & \textrm{with\, probability } \, <  \delta/2 \\
   \notin N_a:  \max \|\bbtheta^k -N_a \| < \epsilon & \textrm{with\, probability } \, < \delta/2 \\
\end{cases}
\]
Implies  either $\bbtheta^k \in N_a$ or $\bbtheta^k \notin N_a$ (for which the probability adds to $\delta$). 
Now using this, we get
\begin{align}
\mathcal{P}^{\bbtheta_0}( \bbtheta_{k\eta} \in N_a) \leq \mathcal{P}^{\bbtheta_0}( \bbtheta^{k} \in N_a) +\delta
\end{align}
\begin{figure}[h]
	%\centering
	%\vspace{4mm}
	{\includegraphics[scale=0.5]{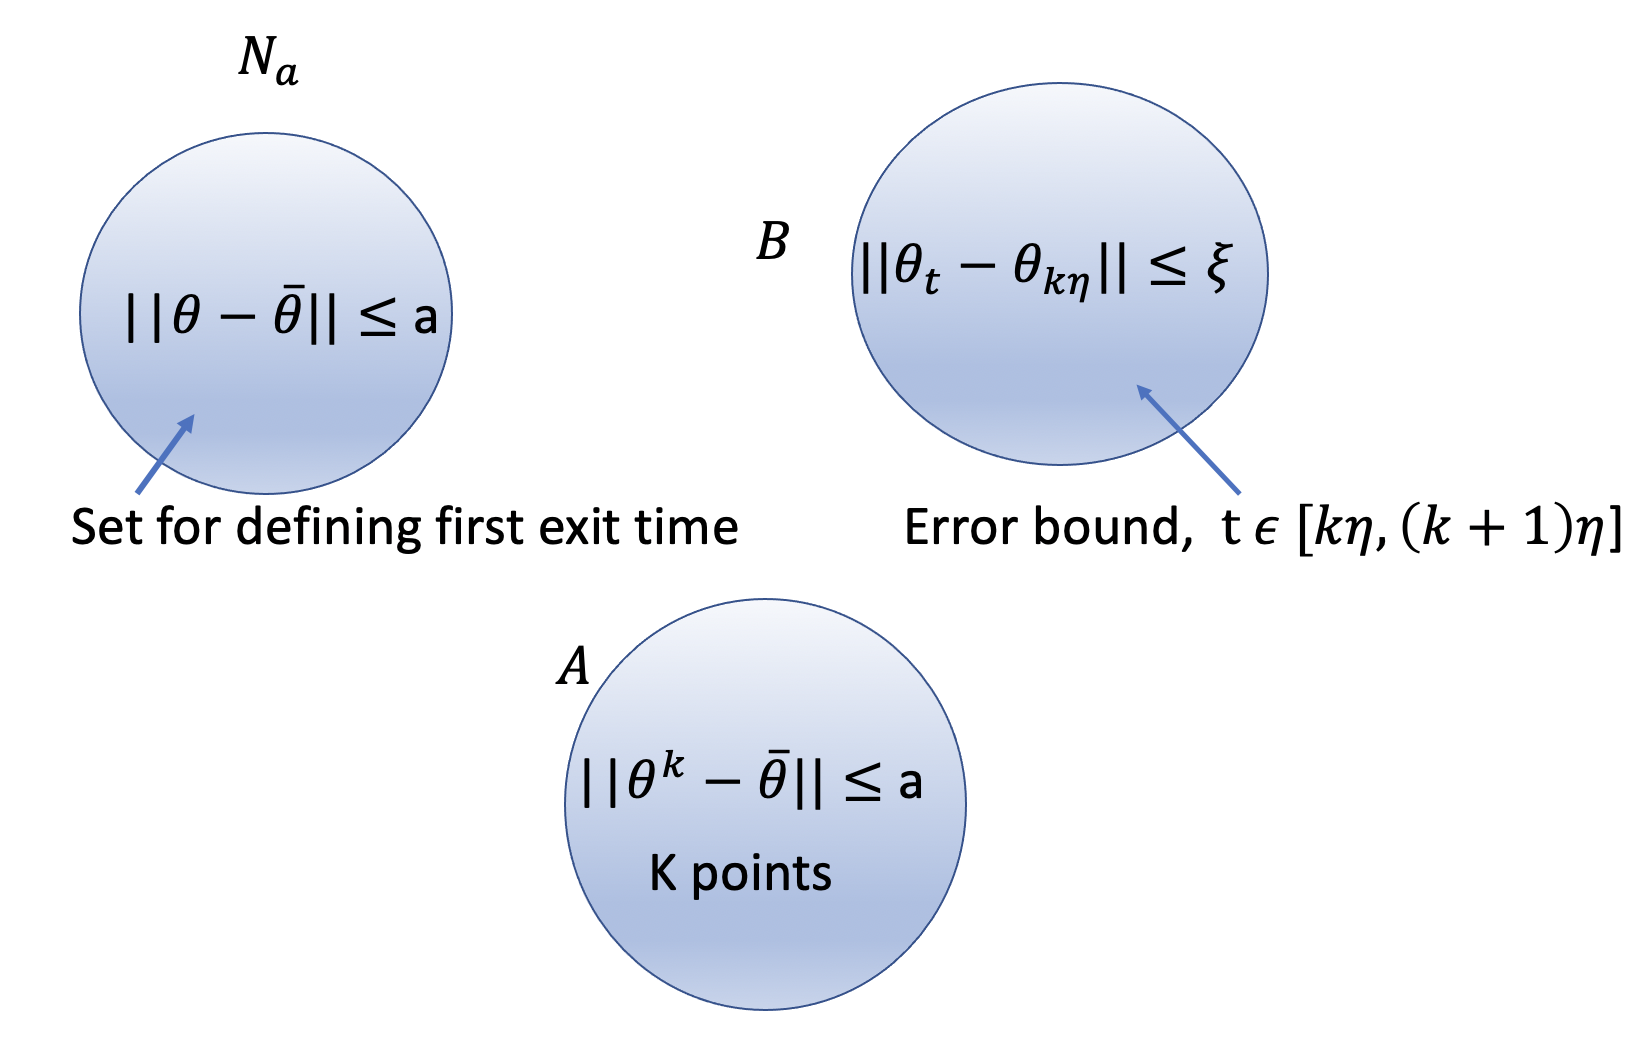}}
	\vspace{0mm}   
	%\centerline{\hspace*{0.6cm}\footnotesize(a)\hspace*{4.3cm}(b)}
	{{\centering  
			\caption{\blue{For mere illustration, we may remove it before submission}} \label{fig:env}}}\vspace{-2mm} 
\end{figure} 
Now probability that $\bbtheta^k \notin N_a$ is $\delta$.   The aforementioned statement can be further extended to the process defined by \eqref{eqn:SGDint} at $t= \eta, \, k\eta, \ldots, ..$ ( as  $\hat{\bbtheta} = \bbtheta^k$ for $\{\hat{\bbtheta}_{s}\}_{ s \in [0, K\eta]}$). We can express the previous statement as
\begin{align}
\mathcal{P}\left( \{ \bbtheta_s \}_{s \in [0, K\eta] } \neq   \{ \hat{\bbtheta}_s\}_{s \in [0, K \eta]}  \right) \leq \delta 
\end{align}
\blue{For the time being, we assume   the processes  \eqref{eqn:SGD_L} and \eqref{eqn:SGD_L1} sampled at discrete instants, $\eta,\, k\eta,\, \ldots..,\,K\eta$ are coupled. Probability that they are not equivalent is upper bounded by some constant, $\delta$. This argument can be proved by evaluating the KL-divergence between the underlying  distributions. And the effect of this argument is bound on the step-size, $\eta$.}   \\
Now analyzing the first exit time of the discrete process. Let $\{ \hat{\bbtheta}_s \in A, \, \textrm{for} \, k=1,\ldots,\, K\}$ and by definition of $A$ and $\bar{\tau}(\cdot)$ from  \eqref{eqn:aset} and \eqref{eqn:taudisccrt},   $\bbtheta^k \in A$ implies  $ \mathcal{P}(\bar{\tau}_{0,a}(\epsilon) > K)$. Therefore,  its continuous equivalent, $\{ \bbtheta_t\} \in A$ or $\{  \bbtheta_t \} \notin A $. And the above statement can be expressed as 
\begin{align}
\mathcal{P}^{\bbtheta_0}\left(  \bar{\tau}_{0,a} (\epsilon) >K) \leq \mathcal{P}^{\bbtheta_0}\left( (\bbtheta_{\eta}, \ldots, \bbtheta_{K\eta} ) \in A    \right)   \right) + \delta
\end{align}
Set, $\left( (\bbtheta_{\eta}, \ldots, \bbtheta_{K\eta} ) \in A    \right) $ implies maximum distance from local minimum is $a$. 
%As we are only aware of the probability of first exit time of continuous SDE from $[0, a +\xi]$, we need to relate $\mathcal{P}^{\bbtheta_0} \left( (\bbtheta_{\eta}, \ldots, \bbtheta_{K\eta} ) \in A    \right) )$ to $\mathcal{P}^{\bbtheta_0}(\hat{\tau}_{\xi,a}(\epsilon) ) $.
 However, we also need to bound the deviation when  $t \in [k\eta, (k+1)\eta]$. In order to do that we ensure that $\|\bbtheta_t-\bbtheta_{k\eta} \| $ is bounded by $\xi$ for the time between $k\eta$ and $(k+1)\eta$. Therefore, we define a set B  such that
\begin{align} \label{eqn:B}
B \triangleq \{   \max_{0 \leq k \leq K-1}  \sup_{t \in [k\eta, (k+1)\eta]} \| \bbtheta_t-\bbtheta_{k\eta} \| \leq \xi  \} 
\end{align} 
Now, the process $[(\bbtheta_{\eta}, \ldots, \bbtheta_{K\eta} ) \in A ] \cap B    )$ ensures that $\bbtheta_t$ is close to $N_a$ for $t= \eta,\ldots, K\eta$.  Let, $ ( \bbtheta_{\eta}, \ldots, \bbtheta_{K\eta}) \in A$, now using the above set we can have two possibilities:for $t \in [k\eta, (k+1) \eta]$, $\|\bbtheta_t-\bbtheta_{k\eta}\|$ can be either in $B$ or outside $B$. Therefore, 
\begin{align}
\mathcal{P}^{\bbtheta_0} ( ( \bbtheta_{\eta}, \ldots, \bbtheta_{K\eta}) \in A) \leq \mathcal{P}^{\bbtheta_0} ( ( \bbtheta_{\eta}, \ldots, \bbtheta_{K\eta}) \in A \cap B ) + \mathcal{P}^{\bbtheta_0}  ( ( \bbtheta_{\eta}, \ldots, \bbtheta_{K\eta}) \in B^c )
\end{align}
First term on the right hand side expression can be expressed as $\mathcal{P}^{\bbtheta_0}(\hat{\tau}_{\xi,a}(\epsilon) \geq K \eta)$. We get, 
\begin{align}
& \mathcal{P}^{\bbtheta_0} \left(  \bar{\tau}_{0,a} (\epsilon) >K\right) \leq  \mathcal{P}^{\bbtheta_0} ( ( \bbtheta_{\eta}, \ldots, \bbtheta_{K\eta}) \in A \cap B ) + \mathcal{P}^{\bbtheta_0} ( ( \bbtheta_{\eta}, \ldots, \bbtheta_{K\eta}) \in B^c ) + \delta \\
& \leq \mathcal{P}^{\bbtheta_0}(\tau_{\xi,a}(\epsilon) \geq K \eta) + \mathcal{P}^{\bbtheta_0} ( ( \bbtheta_{\eta}, \ldots, \bbtheta_{K\eta}) \in B^c ) + \delta 
\end{align}
First inequality is based on the fact that $A \cap B$ defines a domain with its distance from local minima  characterized by $a+\xi$, therefore, first term can be expressed as  $\mathcal{P}(\hat{\tau}_{\xi,a}(\epsilon) \geq K \eta)$.  Now the expression for second term is given by Lemma \ref{lemma:bound}. \\\\\\
Note: Below I outline  two approaches as mentioned in the opening paragraph. \\ Approach 1. Just retain $\mathcal{P}(\hat{\tau}_{\xi,a}(\epsilon) \geq K \eta)$ as given in Mert's paper. In that case, any comments on the exit time except for single dimensional case would be difficult. \\ Approach 2. Relate the above expression to Theorem 3, multi dimensional case.  \\\\
\blue{ Below is the result using first approach: 
\begin{align}
 \mathcal{P}^{\bbtheta_0} \left(  \bar{\tau}_{0,a} (\epsilon) >K\right) 
 \leq &\mathcal{P}(\hat{\tau}_{\xi,a}(\epsilon) \geq K \eta) \nonumber \\
 & + \exp{(M_F \eta)}  M_F \eta  \frac{   C_1  \left( 1 + C_2 \left(\frac{U_R}{(1-\gamma)^2}  (m +b)/2   + C \frac{d}{k_1^{1/\alpha}}   \right)K\eta \right)^{\beta}}{\xi/3}     \nonumber \\
 & +  1- \left(1-C_{\alpha}d^{1+\frac{\alpha}{2}}\eta \exp{(\alpha M\eta)}\epsilon^{\alpha}\left(\frac{\xi}{3}\right)^{-\alpha}\right)^{K} +\delta  
\end{align}
}
Using second approach, we get
\begin{align}
\mathcal{P}^{\bbtheta_0} \left(  \bar{\tau}_{0,a} (\epsilon) >K\right) 
 \leq &\mathcal{P}(\hat{\tau}_{\xi,a}(\epsilon) \geq K \eta) \nonumber \\
 & + \exp{(M_F \eta)}  M_F \eta  \frac{   C_1  \left( 1 + C_2 \left(\frac{U_R}{(1-\gamma)^2}  (m +b)/2   + C \frac{d}{k_1^{1/\alpha}}   \right)K\eta \right)^{\beta}}{\xi/3}    \nonumber \\
 & +  1- \left(1-C_{\alpha}d^{1+\frac{\alpha}{2}}\eta \exp{(\alpha M\eta)}\epsilon^{\alpha}\left(\frac{\xi}{3}\right)^{-\alpha}\right)^{K} +\delta 
  \end{align}
 Let $\bbtheta_0$ in $ \mathcal{G}$,  first term of the above inequality corresponds to the time at which $\bbtheta$ exits $\mathcal{G}$, in other words, time at which  $\bbtheta \in \Omega^{+}(\delta)$.  Therefore
 \begin{align}
 \mathcal{P} \left(  \bar{\tau}_{0,a} (\epsilon) >K\right) 
 \leq &  \mathcal{P}^{\bbtheta_0} \left( \bbtheta_{\hat{\tau}}^{\epsilon}  \in \Omega^{\epsilon+}  \right)  \nonumber \\
 & + \exp{(M_F \eta)}  M_F \eta  \frac{   C_1  \left( 1 + C_2 \left(\frac{U_R}{(1-\gamma)^2}  (m +b)/2   + C \frac{d}{k_1^{1/\alpha}}   \right)K\eta \right)^{\beta}}{\xi/3}     \nonumber \\
 &  +  1- \left(1-C_{\alpha}d^{1+\frac{\alpha}{2}}\eta \exp{(\alpha M\eta)}\epsilon^{\alpha}\left(\frac{\xi}{3}\right)^{-\alpha}\right)^{K} +\delta 
 \end{align}
 where, $\mathcal{P}^{\bbtheta_0} \left( \bbtheta_{\hat{\tau}}^{\epsilon}  \in \Omega^{\epsilon+}  \right) $ indicates the first exit time for a continuous SDE from $\mathcal{G}$.  Now direct application of  Theorem \ref{th:21} for the first term on the right-hand-side of the inequality, we get
 \begin{align}
 \mathcal{P} \left(  \bar{\tau}_{0,a} (\epsilon) >K\right) 
  &\leq  \frac{p^+}{p_s} +  \left[  \exp{(M_F \eta)}  M_F \eta  \frac{   C_1  \left( 1 + C_2 \left(\frac{U_R}{(1-\gamma)^2}  (m +b)/2   + C \frac{d}{k_1^{1/\alpha}}   \right)K\eta \right)^{\beta}}{\xi/3}    \right.  \nonumber \\
 & \left. +  1- \left(1-C_{\alpha}d^{1+\frac{\alpha}{2}}\eta \exp{(\alpha M\eta)}\epsilon^{\alpha}\left(\frac{\xi}{3}\right)^{-\alpha}\right)^{K} +\delta \right]  \\
 &\leq  \frac{p^+}{p_s} +   \mathcal{O} \left( \frac{d}{k_1^{1/\alpha}} K \eta\right)^{\beta}  + \mathcal{O} \left(d^{1+\frac{\alpha}{2}} \exp{(\alpha M\eta)}\epsilon^{\alpha}\left(\frac{\xi}{3}\right)^{-\alpha}\right)^{K}
\end{align}
where,
\begin{align}
& p_s:=  ((d^+)^{-\alpha} + (-d^-)^{-\alpha})\\
& p^+ :=  (d^+)^{-\alpha} \\
& p^- :=  (-d^-)^{-\alpha},
\end{align}
where, $d^+$ and $d^-$ denote distance function to the boundary along unit vector $r$ (cf.  \eqref{eqn:dist}),  $d$ is the dimension of $\bbtheta$, H\"{o}lder continuity constant, $\beta \in (0,1)$, $\delta >0$, $C_{\alpha}>0$, $\xi>0$, $\eta$ is the step-size, $U_R$, $\gamma$ are the parameters of proposed RL setting, positive constants, $C, \, C_1\, C_2$,   are functions of dissipativity constants of score function. 
\\\\
% Analyzing the above expression,  let $\alpha_1<\alpha_2$ and  the first term is greater for $\alpha_1$ for a constants, $C, \epsilon, a$.  Similarly, with $\epsilon/\xi <1$, $0<C_{\alpha}d^{1+\frac{\alpha}{2}}\eta \exp{(\alpha M\eta)}\epsilon^{\alpha}\left(\frac{\xi}{3}\right)^{-\alpha} <1$,  $\left(1-C_{\alpha}d^{1+\frac{\alpha}{2}}\eta \exp{(\alpha M\eta)}\epsilon^{\alpha}\left(\frac{\xi}{3}\right)^{-\alpha}\right)^{K}$ would definitely be of large magnitude for $\alpha_1$. Therefore, for a given basin of interest, we have  high probability  of escape for smaller $\alpha$, in other words, heavier tail. 
\end{proof}
